# Supplementary material for: Information Maximizing Curriculum: A Curriculum-Based Approach for Imitating Diverse Skills
Source: arXiv:2303.15349 source file (2023-10-31)
Supplement: Supplementary file 1 [file ent_pz_fk.tex]

\documentclass{article}
\usepackage{tikz}
\usetikzlibrary{external}
\tikzexternalize[prefix=]

\usepackage{amsmath,amssymb,amsfonts,mathrsfs}
\usepackage{siunitx}
\usepackage{mathtools}

\usepackage[utf8]{inputenc}
\usepackage{pgfplots}
\DeclareUnicodeCharacter{2212}{−}
\usepgfplotslibrary{groupplots,dateplot}
\usetikzlibrary{patterns,shapes.arrows}
\pgfplotsset{compat=newest}
\usetikzlibrary{arrows}
\usepackage{xcolor}

\begin{document}
% This file was created with tikzplotlib v0.10.1.
% This file was created with tikzplotlib v0.10.1.
\begin{tikzpicture}

\definecolor{darkgray176}{RGB}{176,176,176}
\definecolor{steelblue31119180}{RGB}{31,119,180}
\definecolor{darkorange25512714}{RGB}{255,127,14}

\begin{axis}[
tick align=outside,
tick pos=left,
x grid style={darkgray176},
xlabel={\(\displaystyle N_z\)},
xmajorgrids,
xmin=0.5, xmax=200.25,
xtick style={color=black},
y grid style={darkgray176},
ylabel={\(\displaystyle \mathcal{H}(z)\)},
ymajorgrids,
ymin=-0.195513582229614, ymax=5.5,
ytick style={color=black},
legend style={at={(0.995,0.4)}},
    width=0.6\textwidth,
    height=0.35\textwidth,
]
\path [fill=darkorange25512714, opacity=0.3]
(axis cs:1,0)
--(axis cs:1,0)
--(axis cs:5,1.53712072862471)
--(axis cs:10,2.21591259881651)
--(axis cs:25,2.99127448509686)
--(axis cs:50,3.77153620846714)
--(axis cs:75,4.14338095355851)
--(axis cs:100,4.42292403438241)
--(axis cs:125,4.61354188901363)
--(axis cs:150,4.82988631284777)
--(axis cs:175,4.95089942997333)
--(axis cs:200,5.09865551088141)
--(axis cs:200,5.10783373421543)
--(axis cs:200,5.10783373421543)
--(axis cs:175,4.974199624999)
--(axis cs:150,4.8405899648215)
--(axis cs:125,4.6778943063599)
--(axis cs:100,4.44220035017976)
--(axis cs:75,4.16220935812768)
--(axis cs:50,3.80765150261277)
--(axis cs:25,3.08767067481525)
--(axis cs:10,2.24390735383038)
--(axis cs:5,1.59828131503577)
--(axis cs:1,0)
--cycle;

\addplot [ultra thick, darkorange25512714]
table {%
1 0
5 1.56770102183024
10 2.22990997632345
25 3.03947257995605
50 3.78959385553996
75 4.1527951558431
100 4.43256219228109
125 4.64571809768677
150 4.83523813883464
175 4.96254952748617
200 5.10324462254842
};
\addlegendentry{IMC}

\addplot [ultra thick, steelblue31119180]
table {%
1 0
1.66555183946488 0.510156503633966
2.33110367892977 0.846341837369837
2.99665551839465 1.09749683958424
3.66220735785953 1.29806606885991
4.32775919732441 1.46504990167016
4.9933110367893 1.6080992241485
5.65886287625418 1.73322296677548
6.32441471571906 1.84441749526777
6.98996655518395 1.94447577156817
7.65551839464883 2.03542674656188
8.32107023411371 2.11879088046838
8.98662207357859 2.1957370352248
9.65217391304348 2.26718316594313
10.3177257525084 2.3338633629488
10.9832775919732 2.39637389718163
11.6488294314381 2.45520569697531
12.314381270903 2.51076778840234
12.9799331103679 2.56340455797822
13.6454849498328 2.61340869400752
14.3110367892977 2.66103104302613
14.9765886287625 2.70648822376801
15.6421404682274 2.7499685843352
16.3076923076923 2.79163691721048
16.9732441471572 2.8316382305193
17.6387959866221 2.87010079352255
18.304347826087 2.90713861775323
18.9698996655518 2.94285349482128
19.6354515050167 2.9773366826735
20.3010033444816 3.01067031066286
20.9665551839465 3.04292855788328
21.6321070234114 3.07417864730631
22.2976588628763 3.10448168922737
22.9632107023411 3.13389340062695
23.628762541806 3.16246472172794
24.2943143812709 3.19024234689044
24.9598662207358 3.2172691837407
25.6254180602007 3.24358475186991
26.2909698996656 3.26922553040307
26.9565217391304 3.29422526210999
27.6220735785953 3.31861522042003
28.2876254180602 3.34242444464175
28.9531772575251 3.36567994782509
29.61872909699 3.38840690099779
30.2842809364548 3.41062879692683
30.9498327759197 3.43236759607626
31.6153846153846 3.4536438570347
32.2809364548495 3.47447685335424
32.9464882943144 3.49488467846499
33.6120401337793 3.51488434009654
34.2775919732441 3.53449184544088
34.943143812709 3.55372227812553
35.6086956521739 3.57258986792392
36.2742474916388 3.59110805401032
36.9397993311037 3.60928954246353
37.6053511705686 3.62714635863574
38.2709030100334 3.64468989492703
38.9364548494983 3.66193095444099
39.6020066889632 3.67887979094027
40.2675585284281 3.69554614547213
40.933110367893 3.71193927999165
41.5986622073579 3.72806800827315
42.2642140468227 3.74394072436799
42.9297658862876 3.75956542883906
43.5953177257525 3.77494975297692
44.2608695652174 3.79010098118132
44.9264214046823 3.80502607167233
45.5919732441472 3.81973167567841
46.257525083612 3.83422415523402
46.9230769230769 3.84850959970582
47.5886287625418 3.86259384115501
48.2541806020067 3.87648246863274
48.9197324414716 3.8901808414964
49.5852842809365 3.90369410182598
50.2508361204013 3.91702718601272
50.9163879598662 3.9301848355853
51.5819397993311 3.94317160733293
52.247491638796 3.95599188277956
52.9130434782609 3.96864987705838
53.5785953177257 3.98114964723166
54.2441471571906 3.993495100097
54.9096989966555 4.00568999951753
55.5752508361204 4.01773797331053
56.2408026755853 4.02964251972605
56.9063545150502 4.04140701354432
57.5719063545151 4.05303471181873
58.2374581939799 4.0645287592887
58.9030100334448 4.07589219348496
59.5685618729097 4.0871279495481
60.2341137123746 4.09823886477932
60.8996655518395 4.10922768294116
61.5652173913044 4.12009705832452
62.2307692307692 4.13084955959695
62.8963210702341 4.14148767344634
63.561872909699 4.15201380803266
64.2274247491639 4.16243029626014
64.8929765886288 4.17273939888059
65.5585284280937 4.18294330743844
66.2240802675585 4.19304414706711
66.8896321070234 4.20304397914544
67.5551839464883 4.2129448038227
68.2207357859532 4.22274856241978
68.8862876254181 4.23245713971379
69.5518394648829 4.24207236611292
70.2173913043478 4.25159601972761
70.8829431438127 4.2610298283441
71.5484949832776 4.27037547130573
72.2140468227425 4.27963458130715
72.8795986622074 4.28880874610623
73.5451505016722 4.29789951015812
74.2107023411371 4.30690837617573
74.876254180602 4.31583680662056
75.5418060200669 4.32468622512755
76.2073578595318 4.33345801786737
76.8729096989967 4.34215353484964
77.5384615384615 4.35077409116978
78.2040133779264 4.35932096820271
78.8695652173913 4.36779541474593
79.5351170568562 4.37619864811458
80.2006688963211 4.38453185519082
80.866220735786 4.39279619342992
81.5317725752508 4.4009927918251
82.1973244147157 4.40912275183306
82.8628762541806 4.41718714826235
83.5284280936455 4.42518703012607
84.1939799331104 4.43312342146076
84.8595317725753 4.44099732211313
85.5250836120401 4.44880970849593
86.190635451505 4.45656153431463
86.8561872909699 4.46425373126611
87.5217391304348 4.47188720971064
88.1872909698997 4.47946285931851
88.8528428093645 4.48698154969224
89.5183946488294 4.49444413096563
90.1839464882943 4.50185143438064
90.8494983277592 4.509204272843
91.5150501672241 4.51650344145758
92.180602006689 4.5237497180444
92.8461538461538 4.53094386363599
93.5117056856187 4.53808662295706
94.1772575250836 4.54517872488711
94.8428093645485 4.55222088290682
95.5083612040134 4.55921379552873
96.1739130434783 4.56615814671308
96.8394648829431 4.5730546062692
97.505016722408 4.57990383024327
98.1705685618729 4.58670646129276
98.8361204013378 4.59346312904833
99.5016722408027 4.60017445046355
100.167224080268 4.60684103015291
100.832775919732 4.61346346071874
101.498327759197 4.62004232306728
102.163879598662 4.62657818671448
102.829431438127 4.63307161008186
103.494983277592 4.63952314078278
104.160535117057 4.64593331589961
104.826086956522 4.65230266225202
105.491638795987 4.65863169665682
106.157190635451 4.66492092617955
106.822742474916 4.67117084837832
107.488294314381 4.67738195153998
108.153846153846 4.68355471490907
108.819397993311 4.6896896089097
109.484949832776 4.69578709536067
110.150501672241 4.70184762768411
110.816053511706 4.7078716511078
111.481605351171 4.71385960286143
112.147157190635 4.71981191236706
112.8127090301 4.72572900142388
113.478260869565 4.73161128438759
114.14381270903 4.73745916834452
114.809364548495 4.74327305328067
115.47491638796 4.74905333224591
116.140468227425 4.7548003915134
116.80602006689 4.76051461073448
117.471571906355 4.7661963630892
118.137123745819 4.77184601543255
118.802675585284 4.77746392843659
119.468227424749 4.7830504567286
120.133779264214 4.78860594902545
120.799331103679 4.79413074826418
121.464882943144 4.79962519172906
122.130434782609 4.80508961117509
122.795986622074 4.8105243329483
123.461538461538 4.81592967810258
124.127090301003 4.8213059625136
124.792642140468 4.8266534969895
125.458193979933 4.83197258737874
126.123745819398 4.83726353467506
126.789297658863 4.84252663511969
127.454849498328 4.84776218030088
128.120401337793 4.85297045725082
128.785953177258 4.85815174854008
129.451505016722 4.86330633236961
130.117056856187 4.86843448266034
130.782608695652 4.87353646914058
131.448160535117 4.87861255743109
132.113712374582 4.88366300912812
132.779264214047 4.88868808188424
133.444816053512 4.89368802948727
134.110367892977 4.89866310193717
134.775919732441 4.90361354552102
135.441471571906 4.90853960288625
136.107023411371 4.91344151311191
136.772575250836 4.91831951177839
137.438127090301 4.92317383103527
138.103678929766 4.9280046996677
138.769230769231 4.93281234316103
139.434782608696 4.93759698376401
140.100334448161 4.94235884055039
140.765886287625 4.94709812947919
141.43143812709 4.95181506345338
142.096989966555 4.95650985237733
142.76254180602 4.96118270321283
143.428093645485 4.96583382003384
144.09364548495 4.97046340407997
144.759197324415 4.97507165380876
145.42474916388 4.97965876494665
146.090301003344 4.98422493053894
146.755852842809 4.98877034099848
147.421404682274 4.99329518415337
148.086956521739 4.99779964529348
148.752508361204 5.00228390721603
149.418060200669 5.00674815027003
150.083612040134 5.01119255239989
150.749163879599 5.01561728918792
151.414715719064 5.02002253389597
152.080267558528 5.02440845750614
152.745819397993 5.02877522876059
153.411371237458 5.03312301420053
154.076923076923 5.03745197820428
154.742474916388 5.04176228302461
155.408026755853 5.04605408882518
156.073578595318 5.05032755371632
156.739130434783 5.0545828337899
157.404682274248 5.05882008315361
158.070234113712 5.06303945396439
158.735785953177 5.06724109646128
159.401337792642 5.07142515899745
160.066889632107 5.07559178807168
160.732441471572 5.07974112835912
161.397993311037 5.08387332274144
162.063545150502 5.08798851233633
162.729096989967 5.09208683652646
163.394648829431 5.09616843298776
164.060200668896 5.1002334377172
164.725752508361 5.10428198505997
165.391304347826 5.10831420773613
166.056856187291 5.11233023686671
166.722408026756 5.1163302019993
167.387959866221 5.1203142311331
168.053511705686 5.12428245074353
168.719063545151 5.12823498580632
169.384615384615 5.13217195982109
170.05016722408 5.13609349483455
170.715719063545 5.13999971146318
171.38127090301 5.14389072891548
172.046822742475 5.14776666501383
172.71237458194 5.15162763621586
173.377926421405 5.15547375763547
174.04347826087 5.15930514306342
174.709030100334 5.16312190498754
175.374581939799 5.16692415461251
176.040133779264 5.17071200187934
176.705685618729 5.17448555548444
177.371237458194 5.17824492289832
178.036789297659 5.18199021038394
178.702341137124 5.18572152301479
179.367892976589 5.18943896469251
180.033444816054 5.19314263816432
180.698996655518 5.19683264503998
181.364548494983 5.20050908580859
182.030100334448 5.20417205985498
182.695652173913 5.2078216654758
183.361204013378 5.2114579998954
184.026755852843 5.21508115928136
184.692307692308 5.21869123875972
185.357859531773 5.22228833242998
186.023411371237 5.22587253337984
186.688963210702 5.22944393369963
187.354515050167 5.2330026244965
188.020066889632 5.23654869590841
188.685618729097 5.24008223711777
189.351170568562 5.24360333636493
190.016722408027 5.24711208096142
190.682274247492 5.2506085573029
191.347826086957 5.25409285088194
192.013377926421 5.25756504630058
192.678929765886 5.26102522728265
193.344481605351 5.26447347668584
194.010033444816 5.26790987651367
194.675585284281 5.27133450792716
195.341137123746 5.27474745125633
196.006688963211 5.27814878601151
196.672240802676 5.28153859089445
197.33779264214 5.28491694380925
198.003344481605 5.28828392187312
198.66889632107 5.2916396014269
199.334448160535 5.29498405804549
200 5.29831736654804
};
\addlegendentry{$1/N_z$}
\end{axis}

\end{tikzpicture}

\end{document}
