# Supplementary material for: Information Maximizing Curriculum: A Curriculum-Based Approach for Imitating Diverse Skills
Source: arXiv:2303.15349 source file (2023-10-31)
Supplement: Supplementary file 2 [file obs_avoid_ml_cur.tex]

\documentclass{article}
\usepackage{tikz}
\usetikzlibrary{external}
\tikzexternalize[prefix=]

\usepackage{amsmath,amssymb,amsfonts,mathrsfs}
\usepackage{siunitx}
\usepackage{mathtools}

\usepackage[utf8]{inputenc}
\usepackage{pgfplots}
\DeclareUnicodeCharacter{2212}{−}
\usepgfplotslibrary{groupplots,dateplot}
\usetikzlibrary{patterns,shapes.arrows}
\pgfplotsset{compat=newest}
\usetikzlibrary{arrows}
\usepackage{xcolor}

\begin{document}
% This file was created with tikzplotlib v0.10.1.
% This file was created with tikzplotlib v0.10.1.
% This file was created with tikzplotlib v0.10.1.
% [inline block 0: 1 envs, 238021 chars -> data_tex | \begin{tikzpicture} ...]


\end{document}
