# Supplementary material for: Information Maximizing Curriculum: A Curriculum-Based Approach for Imitating Diverse Skills
Source: arXiv:2303.15349 source file (2023-10-31)
Supplement: Supplementary file 5 [file new_result_table.tex]

\newpage
%%%%%%%%%%%%%%%%%%%%%%%%%%%%%%%%%%%%%%%%%%%%%%%%%%%%%%%%%%%%%%%%%%%%%%%
\begin{table*}[t!]
\caption{\scriptsize  \textbf{Result Table}: Performance comparison between various generative models on three behavior learning tasks.}
\label{table:result_table}
\vskip 0.15in
\begin{center}
\begin{small}
\begin{sc}
\resizebox{\textwidth}{!}{%
\begin{tabular}{lcc|ccc|cc}
\toprule
\rule{0pt}{2ex} &
\multicolumn{2}{c}{\textbf{Obstacle Avoidance}} &
\multicolumn{3}{c}{\textbf{Block Pushing}} &
\multicolumn{2}{c}{\textbf{Table Tennis}}  \\
 & 
success rate ($\uparrow$) & Entropy ($\uparrow$) & 
success rate ($\uparrow$) & Entropy ($\uparrow$) & Distance Error ($\downarrow$) & 
success rate ($\uparrow$) & Distance Error ($\downarrow$)\\
\midrule
MDN & 
% ------------------------------------ %
$0.200 \scriptstyle{\pm 0.421}$ &
$0.000 \scriptstyle{\pm 0.000}$ &
% ------------------------------------ %
$ \scriptstyle{\pm }$ &
$ \scriptstyle{\pm }$ &
$ \scriptstyle{\pm }$ &
% ------------------------------------ %
$0.031 \scriptstyle{\pm 0.013}$ &
$0.549 \scriptstyle{\pm 0.056}$ \\
EM & 
% ------------------------------------ %
$0.681 \scriptstyle{\pm 0.049}$ &
$\mathbf{0.910 \scriptstyle{\pm 0.027}}$ &
% ------------------------------------ %
$0.458 \scriptstyle{\pm 0.048}$ &
$0.707 \scriptstyle{\pm 0.042}$ &
$0.127 \scriptstyle{\pm 0.011}$ &
% ------------------------------------ %
$0.725 \scriptstyle{\pm 0.042}$ &
$0.220 \scriptstyle{\pm 0.012}$ \\
DDPM & 
% ------------------------------------ %
$0.719 \scriptstyle{\pm 0.075}$ &
$0.638 \scriptstyle{\pm 0.079}$ &
% ------------------------------------ %
$0.516 \scriptstyle{\pm 0.036}$ & 
$\mathbf{0.713 \scriptstyle{\pm 0.043}}$ &
$0.123 \scriptstyle{\pm 0.007}$ & 
% ------------------------------------ %
$0.866 \scriptstyle{\pm 0.010}$ &
$0.185 \scriptstyle{\pm 0.007}$ \\
NF & 

% ------------------------------------ %
$0.313 \scriptstyle{\pm 0.245}$ &
$0.349 \scriptstyle{\pm 0.208}$ &
% ------------------------------------ %
$ \scriptstyle{\pm }$ &
$ \scriptstyle{\pm }$ &
$ \scriptstyle{\pm }$ &
% ------------------------------------ %
$0.422 \scriptstyle{\pm 0.035}$ &
$0.371 \scriptstyle{\pm 0.013}$ \\
CVAE & 
% ------------------------------------ %
$0.853 \scriptstyle{\pm 0.113}$ &
$0.465 \scriptstyle{\pm 0.183}$ &
% ------------------------------------ %
$0.505 \scriptstyle{\pm 0.089 }$ & 
$0.162 \scriptstyle{\pm 0.071}$  &
$0.123 \scriptstyle{\pm 0.027 }$ & 
% ------------------------------------ %
$0.620 \scriptstyle{\pm 0.050}$ &
$0.320 \scriptstyle{\pm 0.010}$ \\
IBC & 
% ------------------------------------ %
$0.379 \scriptstyle{\pm 0.411}$ &
$0.098 \scriptstyle{\pm 0.131}$ &
% ------------------------------------ %
$0.374 \scriptstyle{\pm 0.041}$ &
$0.607 \scriptstyle{\pm 0.037}$ &
$0.151 \scriptstyle{\pm 0.008}$ &
% ------------------------------------ %
$0.567 \scriptstyle{\pm 0.030}$ &
$0.310 \scriptstyle{\pm 0.010}$ \\
BET & 
% ------------------------------------ %
$0.504 \scriptstyle{\pm 0.076}$ &
$0.837 \scriptstyle{\pm 0.066}$ &
% ------------------------------------ %
$ 0.374\scriptstyle{\pm 0.041}$ &
$ 0.607\scriptstyle{\pm 0.037}$ &
$ 0.151\scriptstyle{\pm 0.008}$ &
% ------------------------------------ %
$0.758 \scriptstyle{\pm 0.025}$ &
$0.235 \scriptstyle{\pm 0.011}$ \\
IMC & 
% ------------------------------------ %
$\mathbf{0.899 \scriptstyle{\pm 0.035}}$ &
${0.887 \scriptstyle{\pm 0.043}}$ &
% ------------------------------------ %
$ \mathbf{0.521\scriptstyle{\pm 0.045}}$ &
$ 0.654\scriptstyle{\pm 0.041}$ &
$ \mathbf{0.120\scriptstyle{\pm 0.014}}$ &
% ------------------------------------ %
$\mathbf{0.870 \scriptstyle{\pm 0.017}}$ &
$\mathbf{0.153 \scriptstyle{\pm 0.007}}$ \\
\bottomrule
\end{tabular}
}
\end{sc}
\end{small}
\end{center}
\vskip -0.1in
\end{table*}
%%%%%%%%%%%%%%%%%%%%%%%%%%%%%%%%%%%%%%%%%%%%%%%%%%%%%%%%%%%%%%%%%%%%%%%
