# Supplementary material for: Information Maximizing Curriculum: A Curriculum-Based Approach for Imitating Diverse Skills
Source: arXiv:2303.15349 source file (2023-10-31)
Supplement: Supplementary file 6 [file obs_avoid_fig.tex]

\section{Further Experiments}
\subsection{Obstacle Avoidance Ablation}
%%%%%%%%%%%%%%%%%%%%%%%%%%%%%%%%%%%%%%%%%%%%%%%%%%%%%%%%%%%%%%%%%%%%%%%
%%%%%%%%%%%%%%%%%%%%%%%%%%%%%%%%%%%%%%%%%%%%%%%%%%%%%%%%%%%%%%%%%%%%%%%
\begin{figure}[t]
\centering
\resizebox{0.14\textwidth}{!}{\includegraphics[width=\textwidth]{supplementary_material/figures/obstacle_avoid_figures/Fig:ICML23:obsavoid_em_1c.pdf}}
\resizebox{0.14\textwidth}{!}{\includegraphics[width=\textwidth]{supplementary_material/figures/obstacle_avoid_figures/Fig:ICML23:obsavoid_em_5c.pdf}}
\resizebox{0.14\textwidth}{!}{\includegraphics[width=\textwidth]{supplementary_material/figures/obstacle_avoid_figures/Fig:ICML23:obsavoid_em_10c.pdf}}
\resizebox{0.14\textwidth}{!}{\includegraphics[width=\textwidth]{supplementary_material/figures/obstacle_avoid_figures/Fig:ICML23:obsavoid_imc_1c.pdf}}
\resizebox{0.14\textwidth}{!}{\includegraphics[width=\textwidth]{supplementary_material/figures/obstacle_avoid_figures/Fig:ICML23:obsavoid_imc_5c.pdf}}
\resizebox{0.14\textwidth}{!}{\includegraphics[width=\textwidth]{supplementary_material/figures/obstacle_avoid_figures/Fig:ICML23:obsavoid_imc_10c.pdf}}
    \caption{\textbf{Obstacle Avoidance Ablation.}
    }
    \label{fig:hbp_ablation}
\end{figure}
